# Supplementary material for: Fast and accurate machine-learned interatomic potentials for large-scale simulations of Cu, Al and Ni
Source: arXiv:2408.15779 source file (2024-08-28)
Supplement: Supplementary file 1 [file supplemental.pdf]

# Supplemental material for: Fast and accurate machine-learned interatomic potentials for large-scale simulations of Cu, Al and Ni

A. Fellman,<sup>1,\*</sup> J. Byggmästar,<sup>1</sup> F. Granberg,<sup>1</sup> K. Nordlund,<sup>1</sup> and F. Djurabekova<sup>1</sup>

<sup>1</sup>*Department of Physics, P.O. Box 43, FI-00014 University of Helsinki, Finland*

(Dated: August 28, 2024)

## S1. BCC AND HCP VOLUME ENERGY CURVES.

In addition to the FCC volume energy curve, in Fig. S1 both the BCC and HCP energy volume curves are shown for all the developed ML potentials. Both the BCC and HCP volume energy curves are in good agreement with DFT results.

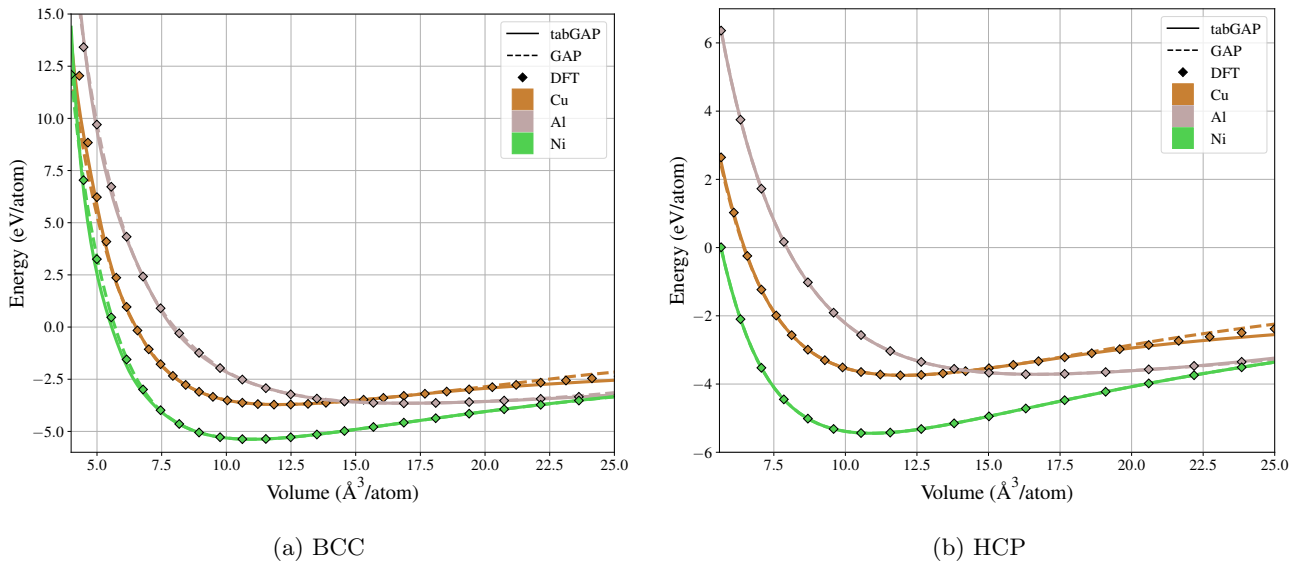

FIG. S1: Energy versus volume curves for BCC (a) and HCP (b).

---

\* Corresponding author; aslak.fellman@helsinki.fi

## S2. UNIAXIAL COMPRESSIVE LOADING IN PRE-DAMAGED COPPER

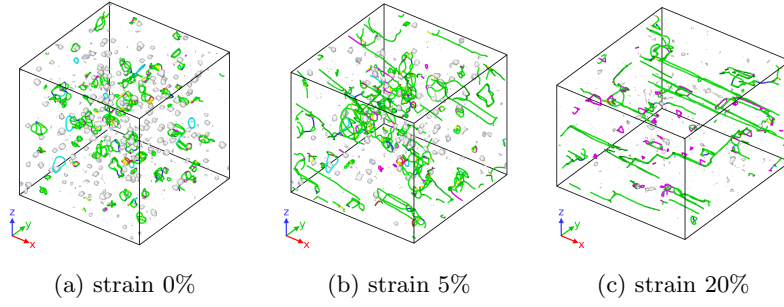

FIG. S2: Cu containing pre-existing defects from Frenkel pair insertion during compression in  $\langle 100 \rangle$  loading direction. Green lines represent Shockley dislocations, cyan lines represent Frank dislocations, pink lines represent stair-rod dislocations, and white blobs are defect clusters that are not identified as dislocations.

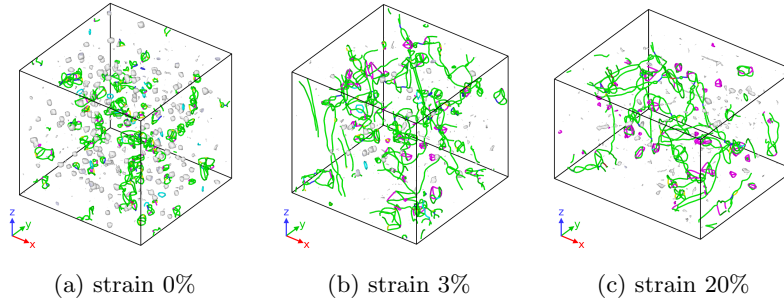

FIG. S3: Cu containing pre-existing defects from Frenkel pair insertion during compression in  $\langle 111 \rangle$  loading direction. Green lines represent Shockley dislocations, cyan lines represent Frank dislocations, pink lines represent stair-rod dislocations, and white blobs are defect clusters that are not identified as dislocations.

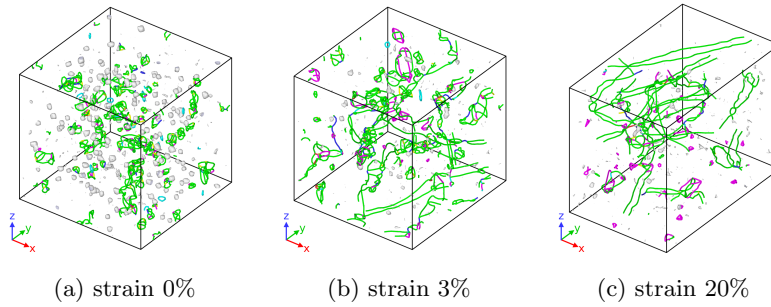

FIG. S4: Cu containing pre-existing defects from Frenkel pair insertion during compression in  $\langle 110 \rangle$  loading direction. Green lines represent Shockley dislocations, cyan lines represent Frank dislocations, pink lines represent stair-rod dislocations, and white blobs are defect clusters that are not identified as dislocations.

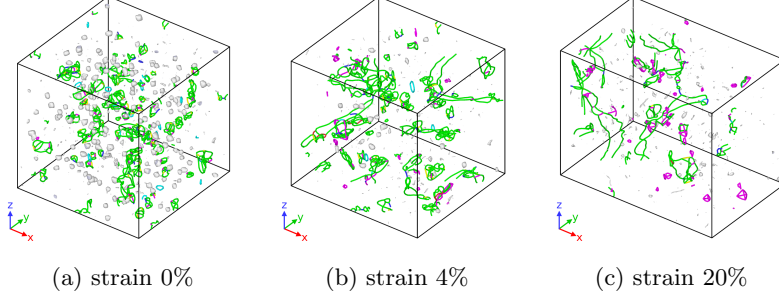

FIG. S5: Cu containing pre-existing defects from Frenkel pair insertion during compression in  $\langle 110 \rangle$  loading direction. Green lines represent Shockley dislocations, cyan lines represent Frank dislocations, pink lines represent stair-rod dislocations, and white blobs are defect clusters that are not identified as dislocations.

### S3. UNIAXIAL COMPRESSIVE LOADING IN PRE-DAMAGED ALUMINIUM

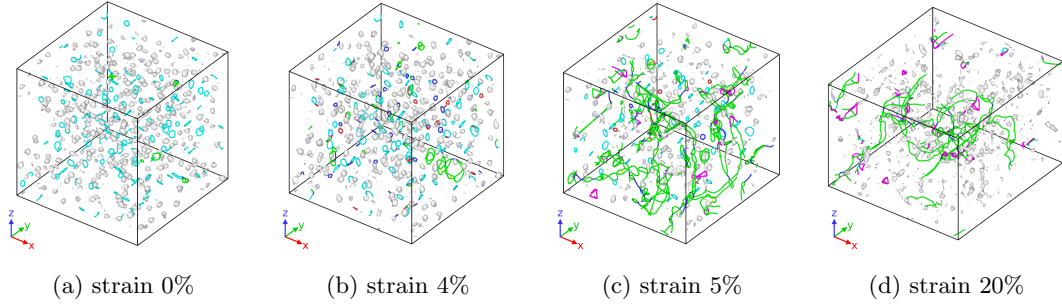

FIG. S6: Al containing pre-existing defects from Frenkel pair insertion during compression in  $\langle 100 \rangle$  loading direction. Green lines represent Shockley dislocations, cyan lines represent Frank dislocations, pink lines represent stair-rod dislocations, and white blobs are defect clusters that are not identified as dislocations.

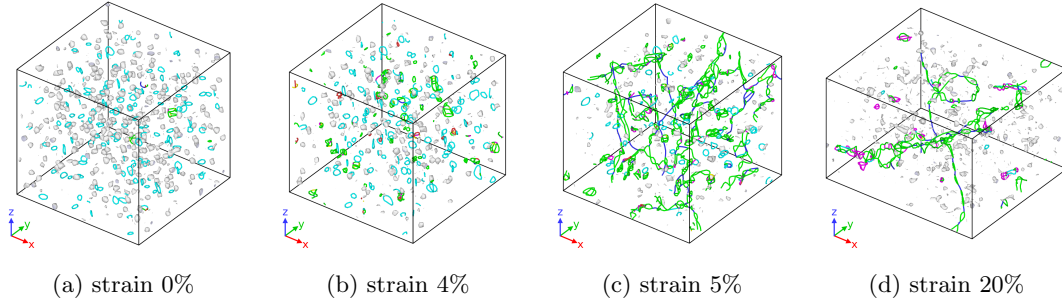

FIG. S7: Al containing pre-existing defects from Frenkel pair insertion during compression in  $\langle 111 \rangle$  loading direction. Green lines represent Shockley dislocations, cyan lines represent Frank dislocations, pink lines represent stair-rod dislocations, and white blobs are defect clusters that are not identified as dislocations.

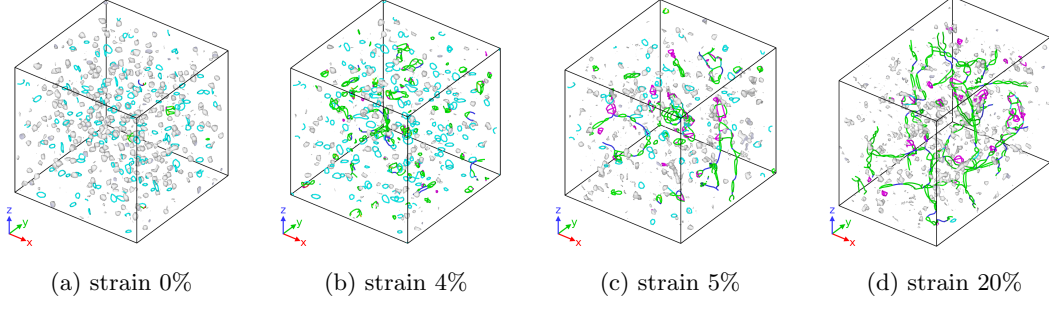

FIG. S8: Al containing pre-existing defects from Frenkel pair insertion during compression in  $\langle 110 \rangle$  loading direction. Green lines represent Shockley dislocations, cyan lines represent Frank dislocations, pink lines represent stair-rod dislocations, and white blobs are defect clusters that are not identified as dislocations.

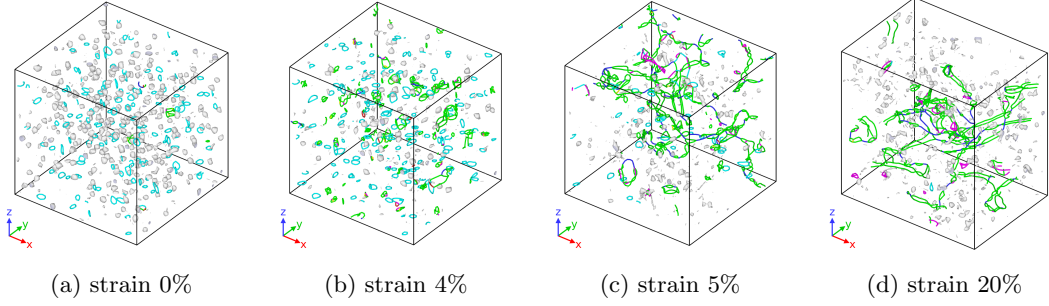

FIG. S9: Al containing pre-existing defects from Frenkel pair insertion during compression in  $\langle 110 \rangle$  loading direction. Green lines represent Shockley dislocations, cyan lines represent Frank dislocations, pink lines represent stair-rod dislocations, and white blobs are defect clusters that are not identified as dislocations.

#### S4. UNIAXIAL COMPRESSIVE LOADING IN PRE-DAMAGED NICKEL

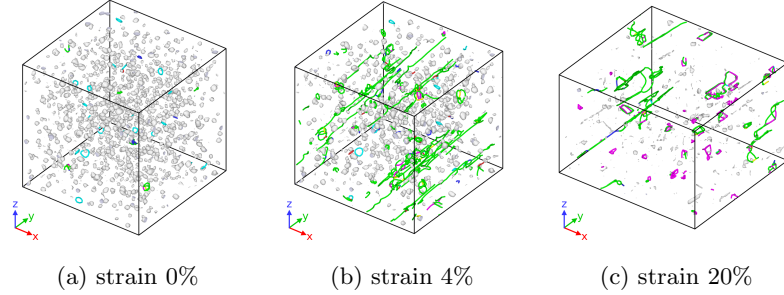

FIG. S10: Ni containing pre-existing defects from Frenkel pair insertion during compression in  $\langle 100 \rangle$  loading direction. Green lines represent Shockley dislocations, cyan lines represent Frank dislocations, pink lines represent stair-rod dislocations, and white blobs are defect clusters that are not identified as dislocations.



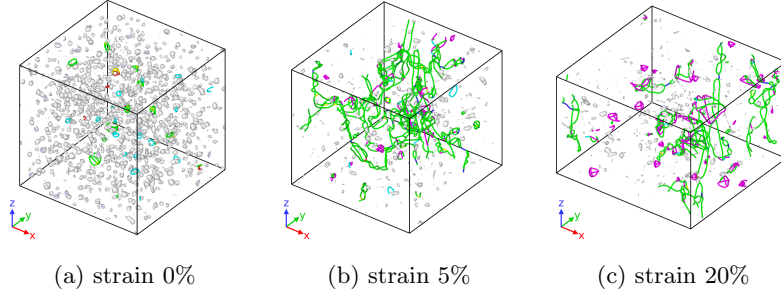

FIG. S11: Ni containing pre-existing defects from Frenkel pair insertion during compression in  $\langle 111 \rangle$  loading direction. Green lines represent Shockley dislocations, cyan lines represent Frank dislocations, pink lines represent stair-rod dislocations, and white blobs are defect clusters that are not identified as dislocations.

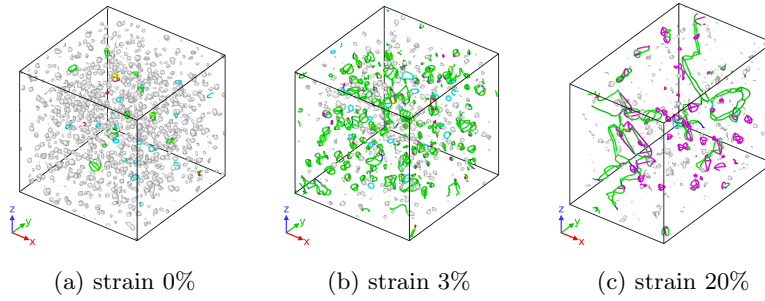

FIG. S12: Ni containing pre-existing defects from Frenkel pair insertion during compression in  $\langle 110 \rangle$  loading direction. Green lines represent Shockley dislocations, cyan lines represent Frank dislocations, pink lines represent stair-rod dislocations, and white blobs are defect clusters that are not identified as dislocations.

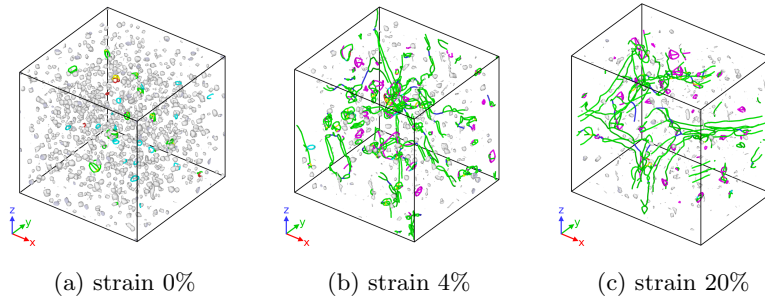

FIG. S13: Ni containing pre-existing defects from Frenkel pair insertion during compression in  $\langle 110 \rangle$  loading direction. Green lines represent Shockley dislocations, cyan lines represent Frank dislocations, pink lines represent stair-rod dislocations, and white blobs are defect clusters that are not identified as dislocations.
